# Supplementary material for: Strengthening Skeletal Action Recognizers via Leveraging Temporal Patterns
Source: arXiv:2205.14405 source file (2022-08-23)
Supplement: Supplementary file 1 [file limitation.tex]

\section{Limitations}
Both \encabbr{} and \losabbr{} additionally add slightly more parameters and inference time. As shown in \textcolor{blue}{Table~1} of the main paper, the number of parameters (in millions) for BKB is 1.44. \encabbr{} increases this number to 1.46, and \losabbr{} enlarges the value to 1.77. As for the inference time, the GFlops of BKB is 19.4. Both \encabbr{} and \losabbr{} expand the value to be 19.6. 

One may worry that the accuracy improvement may result from these additional parameters and inference time rather than the proposed methods. Here, we experimentally dispel these worrying cases. 

To begin with, as we have shown in section 4.3 of the main paper, we have tried two other approaches of enlarging the input feature dimension: 
1) The extended dimensional values are the elementwise product of the randomly generated values between $-1$ and $1$ and the original sequence; the range between $-1$ and $1$ coincides with the cosine's amplitude. 2) The enlarged dimensions are the simple repetition of the original skeleton 3D coordinates. Although these two methods introduce the same amount of the additional number of parameters and GFlops as \encabbr{} does, neither of these two ways improves the accuracy. 

Furthermore, we have also evaluated the accuracy by enlarging the number of parameters by increasing the dimensions of hidden layers. We double the dimension of each hidden representation. This leads to that the number of parameters increases from 1.44 M to 6.93 M and the inference GFlops enlarges from 19.4 to 77.62. However, the recognition accuracy does not improve. This implies that the accuracy improvement does not come from the additional parameters.
