# Supplementary material for: Strengthening Skeletal Action Recognizers via Leveraging Temporal Patterns
Source: arXiv:2205.14405 source file (2022-08-23)
Supplement: Supplementary file 2 [file more_exp.tex]

\section{More Experiments}
\subsection{Comparison with Rank Pooling}
CRL consistently outperforms the rank pooling loss~\cite{2016_cvpr_rank_pooling}, as shown in \autoref{tab:11_crl_compare}.
%\autoref{tab:11_crl_compare} shows the comparison between rank pooling in [11] and CRL. CRL consistently outperforms rank pooling. 
We conjecture that CRL's higher accuracy is because the rank pooling loss linearly transforms the features of each frame while CRL transfers each frame’s representation using a neural network with non-linear activation. Previous work has revealed that non-linear activation enhances a model’s capability~\cite{lu2017expressive}. 

\begin{table}[h!]\small
\centering
\caption{
Comparison between the rank pooling in~\cite{2016_cvpr_rank_pooling} and CRL. 
}
% \vspace{-2mm}
% \resizebox{\linewidth}{!}{
\begin{tabular}{l c | rr  rr }
\toprule
% row 1
%\rowcolor{Gray}
&
&
\multicolumn{2}{c }{\textbf{NTU60}} 
& \multicolumn{2}{c}{\textbf{NTU120}}
% & \multicolumn{2}{c }{\textbf{Kinetics}}
\\
% row 2
\cline{3-6}
%\rowcolor{Gray}
\multirow{-2}{*}{\textbf{Methods}} &
\multirow{-2}{*}{\textbf{Features}}  &
X-Sub
& X-View
& X-Sub
& X-Set
% & Top-1 & Top-5 
\\
\midrule 
Rank Pooling & Joint & 87.6 & 93.7 & 82.1 & 84.0 \\
CRL & Joint & 88.2 & 95.2 & 82.5 & 84.3 \\
\midrule 
Rank Pooling & Bone & 88.6 & 94.0 & 84.4 & 85.8 \\
CRL & Bone & 89.4 & 95.3 & 84.7 & 86.6 \\
\bottomrule
\end{tabular}
% }
\label{tab:11_crl_compare}
\end{table}

\subsection{DCE Without the Original Sequence}
The results of DCE without concatenating with the original sequence are shown in \autoref{tab:no_concat}. Concatenating frequency features with original features leads to higher accuracy.

\begin{table}[h!]\small
\centering
\caption{
Results of DCE without and with the original sequence. 
}
% \resizebox{\linewidth}{!}{
\begin{tabular}{l c | rr  rr }
\toprule
% row 1
%\rowcolor{Gray}
&
&
\multicolumn{2}{c }{\textbf{NTU60}} 
& \multicolumn{2}{c}{\textbf{NTU120}}
% & \multicolumn{2}{c }{\textbf{Kinetics}}
\\
% row 2
\cline{3-6}
%\rowcolor{Gray}
\multirow{-2}{*}{\textbf{Methods}} &
\multirow{-2}{*}{\textbf{Features}}  &
X-Sub
& X-View
& X-Sub
& X-Set
% & Top-1 & Top-5 
\\
\midrule 
No-Concat & Joint & 88.0 & 94.3 & 82.5 & 83.6 \\
With-Concat & Joint & 88.5 & 95.0 & 83.1 & 85.1 \\
\midrule 
No-Concat & Bone & 89.7 & 94.8 & 85.1 & 86.1 \\
With-Concat & Bone & 90.0 & 95.1 & 85.5 & 86.6 \\
\bottomrule
\end{tabular}
% }
\label{tab:no_concat}
\end{table}

\subsection{Studies of different $K$}
We found accuracy improves as K grows, as one further example is given in \autoref{tab:diff_K}. 

\begin{table}[h!]\small
\centering
% \vspace{-2mm}
\caption{
Results of $K = 8$ and $K=12$. 
% \dw{(Try to add the result of K=8 such that the reviewer can check the difference without reading the submitted one again. However, on the other hand, the question is more about ablation, so including these results may weaker our experiments - since the reviewer thinks we did not perform proper search for the hyperparameters.)}
} 
% \resizebox{0.8\linewidth}{!}{
\begin{tabular}{l c | rr  rr }
\toprule
% row 1
%\rowcolor{Gray}
&
&
\multicolumn{2}{c }{\textbf{NTU60}} 
& \multicolumn{2}{c}{\textbf{NTU120}}
% & \multicolumn{2}{c }{\textbf{Kinetics}}
\\
% row 2
\cline{3-6}
%\rowcolor{Gray}
\multirow{-2}{*}{\textbf{$K$}} &
\multirow{-2}{*}{\textbf{Features}}  &
X-Sub
& X-View
& X-Sub
& X-Set
% & Top-1 & Top-5 
\\
\midrule 
8 & Joint & 88.5 & 95.0 & 83.1 & 85.1 \\
12 & Joint & 88.7 & 95.1 & 83.4 & 85.3 \\
\midrule 
8 & Bone & 90.0 & 95.1 & 85.5 & 86.6 \\
12 & Bone & 90.1 & 95.1 & 85.9 & 86.7 \\
\bottomrule
\end{tabular}
% }
\label{tab:diff_K}
\end{table}
