# Supplementary material for: Strengthening Skeletal Action Recognizers via Leveraging Temporal Patterns
Source: arXiv:2205.14405 source file (2022-08-23)
Supplement: Supplementary file 3 [file visual.tex]

\begin{figure*}[t]
\centering
\begin{subfigure}{.99\textwidth}
  \centering
  \includegraphics[width=0.7\linewidth]{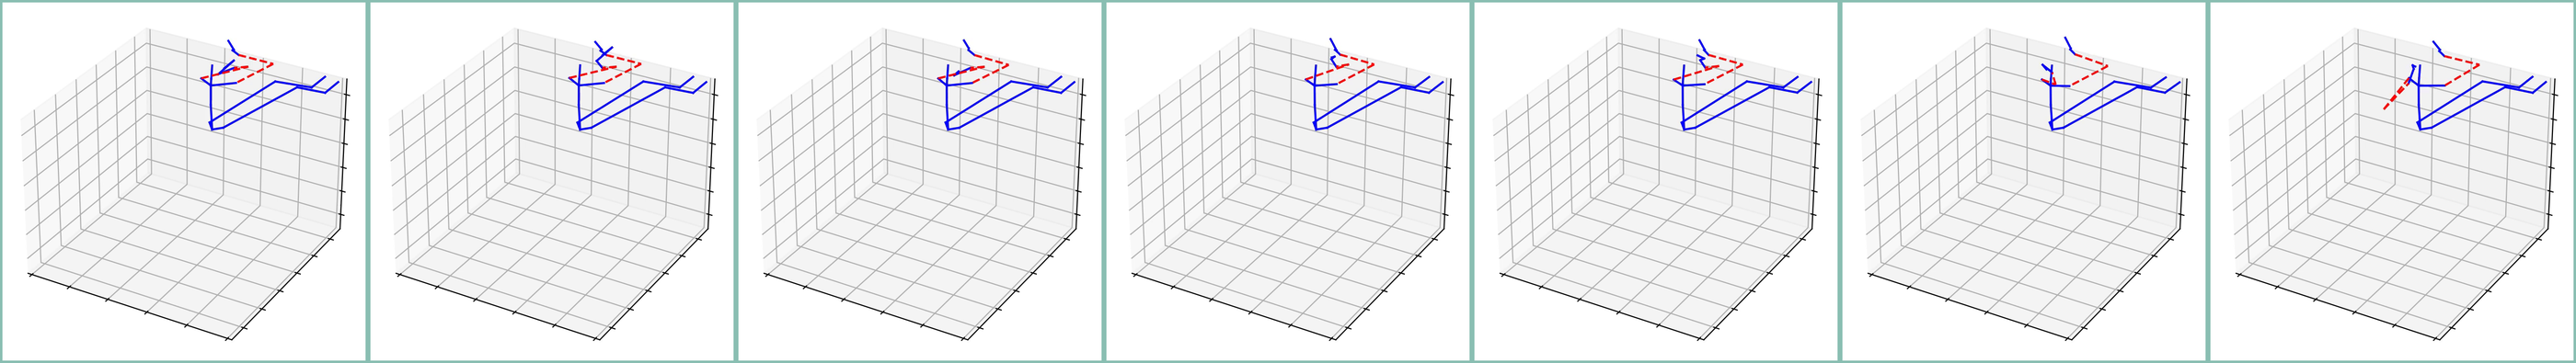}
\end{subfigure}

\begin{subfigure}{.99\textwidth}
  \centering
  \includegraphics[width=0.7\linewidth]{imgs/A003RGB.png}
%   \vspace{-6mm}
  \subcaption{\textbf{Brushing teeth}. The estimated joints of the elbows and hands are jumping around. The baseline model recognizes the input wrongly as \enquote{writing}. \encabbr{} corrects the prediction and increases the confidence to the GT label (\enquote{brush teeth}) from 0.03 to 0.47. }
  \label{subfig:tte_brushing_teeth}
%   \vspace{1mm}
\end{subfigure}

\begin{subfigure}{.99\textwidth}
  \centering
  \includegraphics[width=0.7\linewidth]{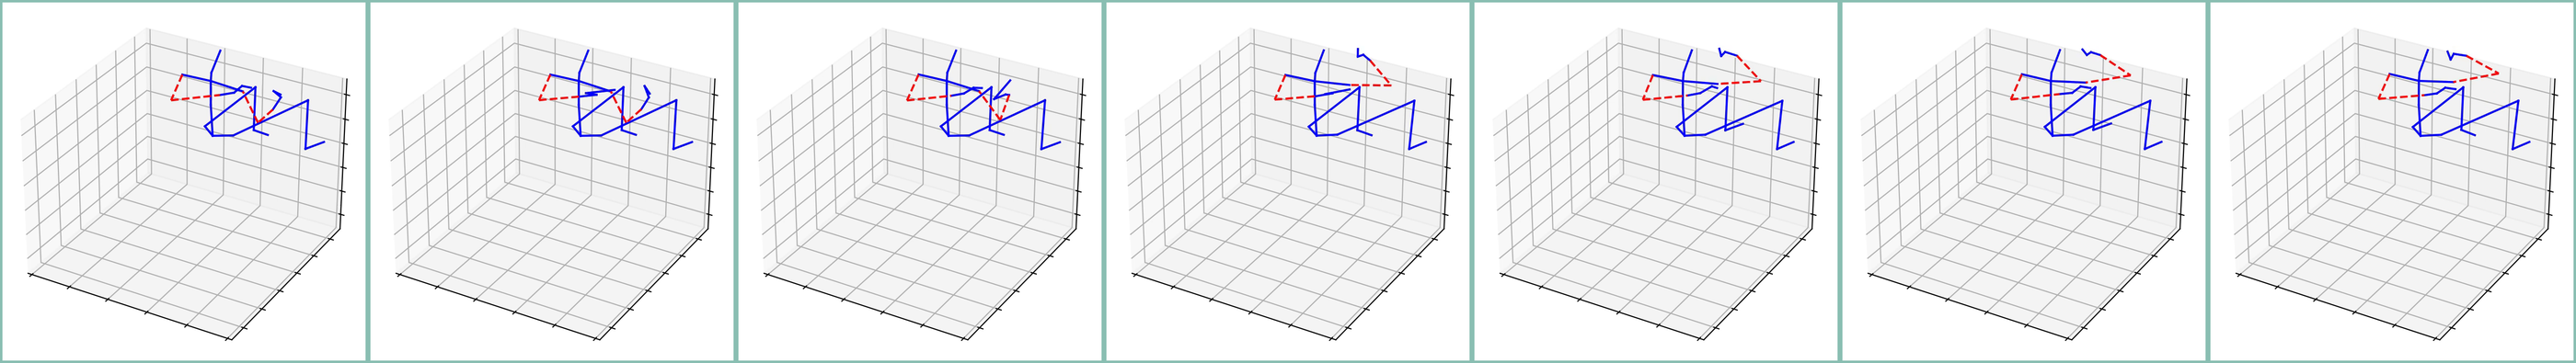}
\end{subfigure}

\begin{subfigure}{.99\textwidth}
  \centering
  \includegraphics[width=0.7\linewidth]{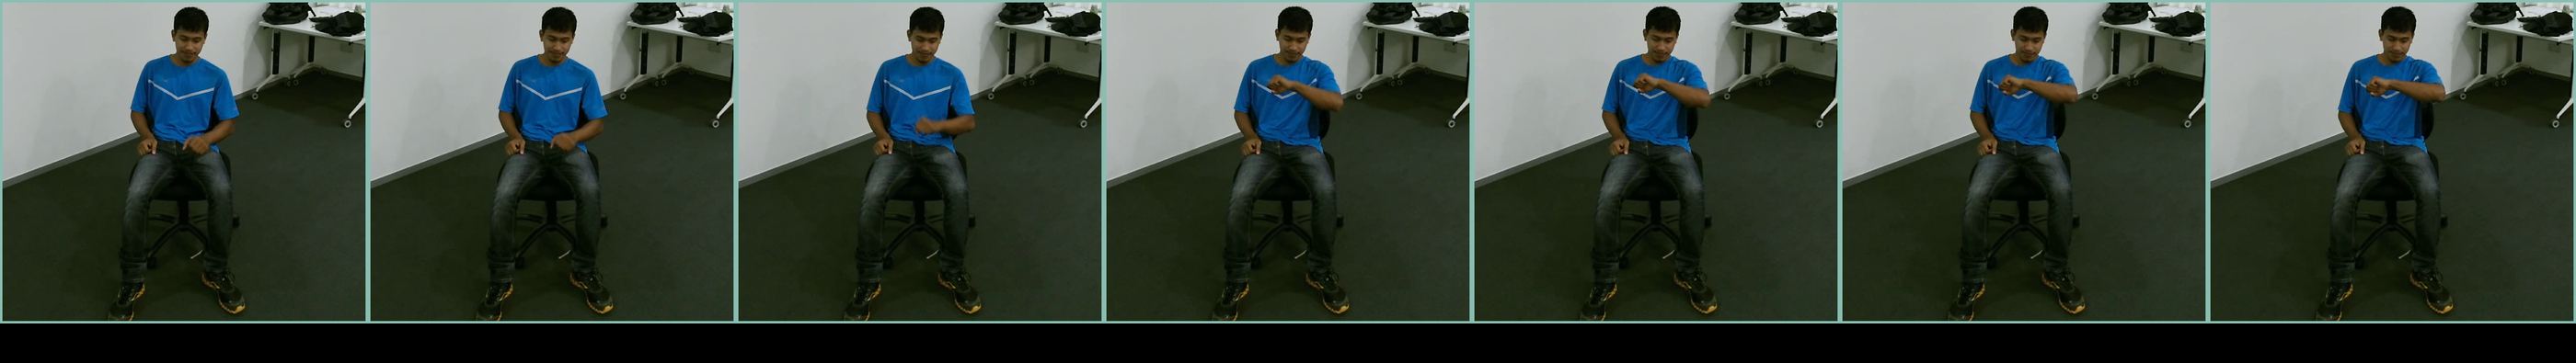}
%   \vspace{-6mm}
  \subcaption{\textbf{Checking time (from watch)}. The estimated skeletons contain much fake jittering of hands and feet. The baseline model recognizes the input wrongly as \enquote{eat meal/snack}. \encabbr{} corrects the prediction and increases the confidence to the GT label (\enquote{checking time (from watch)}) from 0.07 to 0.51.}
%   \vspace{1mm}
\end{subfigure}

\begin{subfigure}{.99\textwidth}
  \centering
  \includegraphics[width=0.7\linewidth]{imgs/A001Skeleton.png}
\end{subfigure}

\begin{subfigure}{.99\textwidth}
  \centering
  \includegraphics[width=0.7\linewidth]{imgs/A001RGB.png}
%   \vspace{-6mm}
  \subcaption{\textbf{Drinking water}. The estimated forearm unrealistically hangs on the elbow and rotates around and swings back and forth in a physically-impossible fashion. The baseline model recognizes the input wrongly as \enquote{make a phone call}. \encabbr{} corrects the prediction and increases the confidence to the GT label (\enquote{drink water}) from 0.01 to 0.70.}
%   \vspace{1mm}
\end{subfigure}

\begin{subfigure}{.99\textwidth}
  \centering
  \includegraphics[width=0.7\linewidth]{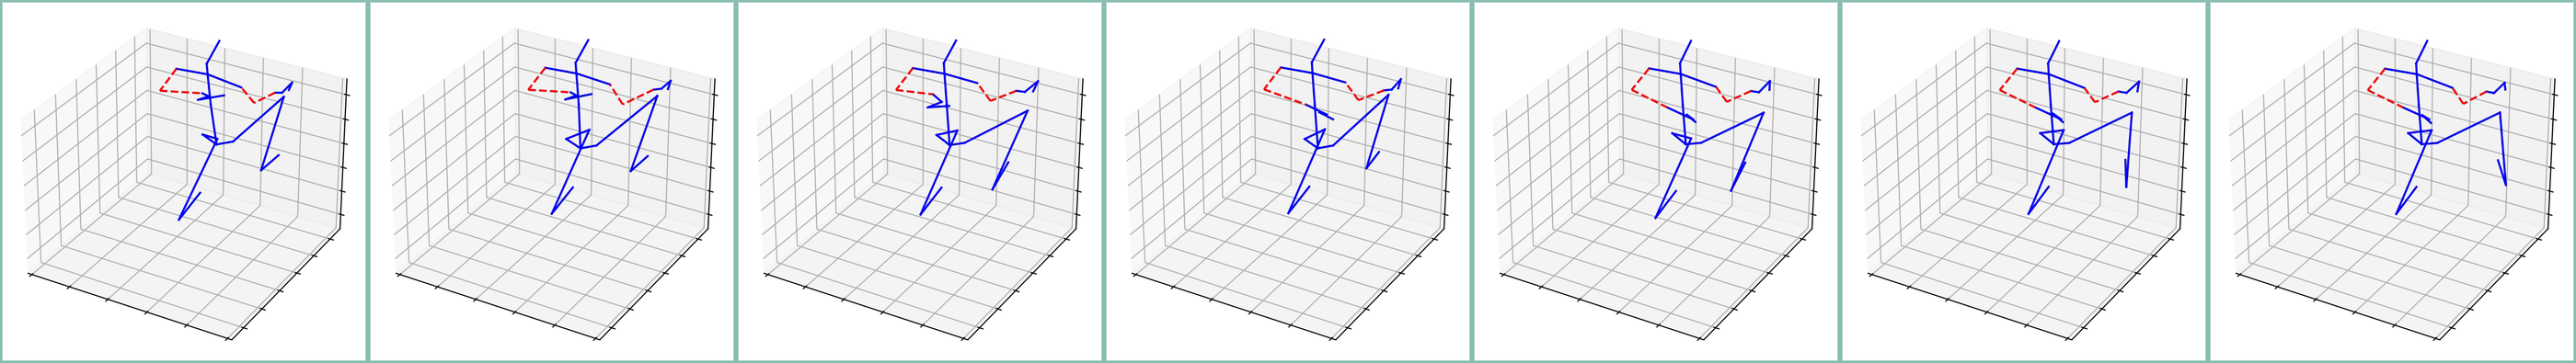}
\end{subfigure}

\begin{subfigure}{.99\textwidth}
  \centering
  \includegraphics[width=0.7\linewidth]{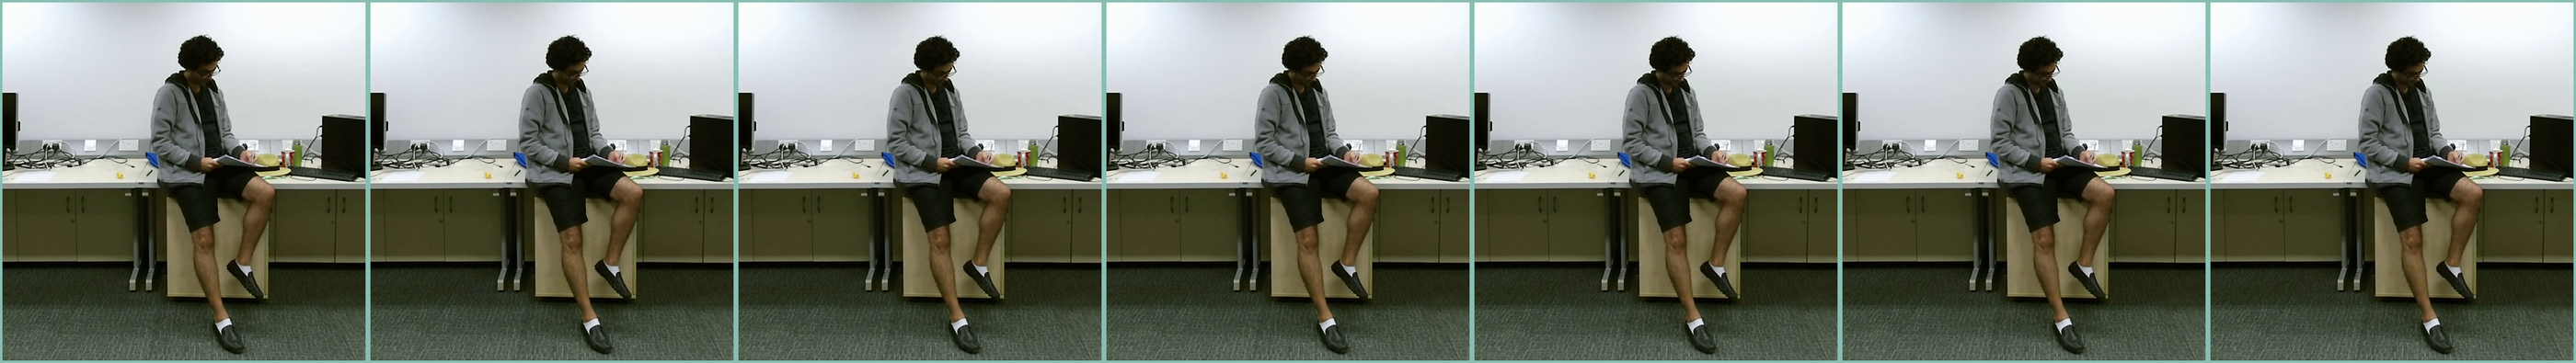}
%   \vspace{-1mm}
  \subcaption{\textbf{Writing}. The skeletons for the legs and the hands contain fake drastic movements. The baseline model recognizes the input wrongly as \enquote{type on a keyboard}. \encabbr{} corrects the prediction and increases the confidence to the GT (\enquote{writing}) label from 0.02 to 0.50. }
  \end{subfigure}
\caption{Visual examples of challenging skeleton actions whose predictions are rectified by \encabbr{}. Best viewed with high-resolution screens with zoom-in. The second row contains the corresponding RGB frames (usually from a different view).}
\label{fig:noise_sample_TTE}
% \vspace{-2mm}
\end{figure*}

\section{Visualized Samples}
Skeleton actions can be challenging to recognize due to their noise. We classify the challenging noisy skeleton videos into three types: (1) having fake local joint oscillation; (2) containing wrongly estimated human poses; (3) with incomplete skeletons due to occlusion.

As shown in~\autoref{fig:noise_sample_TTE}, \encabbr{} can resist all the three kinds of challenges in skeleton videos by temporally smoothing out the noise. 
Before using \encabbr{}, the baseline model predicts wrong labels for the videos illustrated in~\autoref{fig:noise_sample_TTE}. In contrast, after employing \encabbr{}, the model is able to recognize the actions accurately.
