# Supplementary material for: Strengthening Skeletal Action Recognizers via Leveraging Temporal Patterns
Source: arXiv:2205.14405 source file (2022-08-23)
Supplement: Supplementary file 4 [file assets.tex]

\section{Use of Existing Assets}
We utilize the publicly available benchmarking datasets for fairly evaluating and comparing our methods with others. The datasets are NTU60~\cite{2016_cvpr_ntu} and NTU120~\cite{2019_tpami_ntu120}. We obtain the datasets through the website of~\cite{ntu_dataset_website}. Refer to the website for more details such as the license information.
