# Supplementary material for: Strengthening Skeletal Action Recognizers via Leveraging Temporal Patterns
Source: arXiv:2205.14405 source file (2022-08-23)
Supplement: Supplementary file 5 [file backbone.tex]

% \begin{figure*}
%     \centering
%     \includegraphics[width=\linewidth]{imgs/backbone.png}
%     \caption{
%     Illustration of the utilized backbone architecture. It consists of three spatial temporal units (STUs). Each STU constitutes a spatial feature extractor (SFE) and three temporal pattern extractors (TPEs). The SFE captures spatial interactions with parallel graph convolutional branches. The TPE draws temporal patterns with several functional components. 
%     }
%     \label{fig:backbone}
% \end{figure*}

\section{Backbone}
% We apply a simplified MS-G3D~\cite{2020_cvpr_msg3d} as the backbone of our model. The simplicity lies on the removal of the computationally heavy G3D component. Empirically, this leads to the inference time to become 40\% of the original. The backbone's illustration is pictorially depicted in \autoref{fig:backbone}. The skeleton sequence sequentially passes through three spatial-temporal units (STUs), as exhibited in \autoref{fig:backbone}(a). An STU consists of a spatial feature extractor (SFE) and three temporal pattern extractors (TPEs).

We apply a simplified MS-G3D~\cite{2020_cvpr_msg3d} as the backbone of our model. The simplicity lies in the removal of the computationally heavy G3D component. Empirically, this leads the inference time becoming 40\% of the original. The skeleton sequence passes through three spatial-temporal units sequentially (STUs). An STU consists of a spatial feature extractor (SFE) and three temporal pattern extractors (TPEs).
