# Supplementary material for: Strengthening Skeletal Action Recognizers via Leveraging Temporal Patterns
Source: arXiv:2205.14405 source file (2022-08-23)
Supplement: Supplementary file 7 [file human.tex]

\section{Personal Data/Human Subjects}
Refer to~\cite{2019_tpami_ntu120} for more details about the consent information, subject information, and the collection procedures.
