# Supplementary material for: Strengthening Skeletal Action Recognizers via Leveraging Temporal Patterns
Source: arXiv:2205.14405 source file (2022-08-23)
Supplement: Supplementary file 8 [file impact.tex]

\section{Potential Negative Impact}
People may concern about the privacy issues of recognizing human actions. We argue that compared with the RGB modal, it is challenging to exploit personal identity information using skeleton sequences. This is because sensitive features such as faces or clothing visual cues are absent in skeletonized human representations. We also further disguise the individual differences by normalizing skeletons to be of the same size.
